# Supplementary material for: All-optical convolution utilizing processing in memory based on a cold atomic ensemble
Source: arXiv:2506.14716 source file (2025-06-17)
Supplement: Supplementary file 1 [file supplemental.pdf]

# Supplemental Material for All-optical convolution utilizing processing in memory based on a cold atomic ensemble

Ying-Hao Ye,[1,2,3] Jia-Qi Jiang,[4] En-Ze Li,[1,2,3] Wei Zhang,[1,2,3] Da-Chuang Li,[5] Zhi-Han Zhu,[4,*] Dong-Sheng Ding,[1,2,3,†] and Bao-Sen Shi[1,2,3,‡]

[1]*Anhui Province Key Laboratory of Quantum Network, University of Science and Technology of China, Hefei 230026, China.*
[2]*Laboratory of Quantum Information, University of Science and Technology of China, Hefei 230026, China.*
[3]*Hefei National Laboratory, University of Science and Technology of China, Hefei 230088, China.*
[4]*Wang Da-Heng Center, Heilongjiang Key Laboratory of Quantum Control, Harbin University of Science and Technology, Harbin 150080, China.*
[5]*Institute for Quantum Control and Quantum Information and School of Physics and Materials Engineering, Hefei Normal University, Hefei, Anhui 230601, China*

## I. CONVERSION OF SPIRAL PHASES BETWEEN CONTROL FIELD AND ATOMIC COLLECTIVE EXCITATIONS

The essence of the proposed PIM scheme is conversion of spiral phases between control fields and atomic collective excitation. Following the conventional method of master equations [1], the evolution of light-matter system in the presence of a weak signal field and a strong control field with vortex phase can be described by the following equations (the arguments of the operators are indicated only where it is necessary to emphasize their presence):

$$\left(\frac{\partial}{\partial t}+c\frac{\partial}{\partial z}-\frac{ic}{2k_s}\frac{\partial^2}{\partial\rho^2}\right)\hat{a}_f\left(\vec{\rho},z,t\right)=igN\hat{\sigma}_{ge}, \tag{S1a}$$

$$\dot{\hat{\sigma}}_{ge}=ig\left(\hat{\sigma}_{gg}-\hat{\sigma}_{ee}\right)\hat{a}_f+i\Omega\mathcal{U}_l\hat{\sigma}_{gs}, \tag{S1b}$$

$$\dot{\hat{\sigma}}_{gs}=i\Omega^*\mathcal{U}_l^*\hat{\sigma}_{ge}-ig\hat{a}_f\hat{\sigma}_{es}. \tag{S1c}$$

Here $\hat{\sigma}_{\mu\nu}$ is a slowly varying continuous atomic flip operator from $|\nu\rangle$ to $|\mu\rangle$, $\vec{\rho}$ refers to the transverse coordinate, $N$ denotes the number of atoms in the interacting region and $g$ represents the atom-field coupling strength. $\hat{a}_f\left(\vec{\rho},z,t\right)$ is a spatially resolved annihilation operator for signal photon, with its distribution determined by the pattern mask (FIG. 1 (b) in the maintext). Since the expanded control field has a much larger radius than that of the signal field, we assume that the coupling field is a quasimonochromatic quasiplane wave with Rabi frequency $\Omega\left(t\right)$ and then multiply it with a spiral phase $\mathcal{U}_l=e^{il\phi}$, where $\phi$ is the azimuth angle and obviously $\mathcal{U}_l^{-1}=\mathcal{U}_l^*=\mathcal{U}_{-l}$. We have disregarded all the transversal or longitudinal decay terms and Langevin noise terms Eqs. 1 for the sake of simplicity.

When the Rabi frequency of signal pulse is much smaller than $\Omega$ and has a much lower number density of photons compared to that of atoms, the only non-zero diagonal term in the lowest order approximation is $\hat{\sigma}_{gg}=1$. We then rotate the reference frame as $\tilde{\sigma}_{gs}=\hat{\sigma}_{gs}\mathcal{U}_l$, $\tilde{\sigma}_{ge}=\hat{\sigma}_{ge}$ and obtain a more concise form:

$$\tilde{\sigma}_{gs}=-i\dot{\tilde{\sigma}}_{ge}/\Omega-g\hat{a}_f/\Omega, \tag{S2a}$$

$$\tilde{\sigma}_{ge}=-i\dot{\tilde{\sigma}}_{gs}/\Omega^*. \tag{S2b}$$

In a bid to solve Eqs. 2 when $\dot{\Omega}\neq 0$, the concept of dark state polariton (DSP) is introduced as:

$$\hat{\Psi}=\cos\theta\left(t\right)\hat{a}_f-\sin\theta\left(t\right)\sqrt{N}\tilde{\sigma}_{gs}, \tag{S3a}$$

$$\hat{\Phi}=\sin\theta\left(t\right)\hat{a}_f+\cos\theta\left(t\right)\sqrt{N}\tilde{\sigma}_{gs}. \tag{S3b}$$

* zhuzhihan@hrbust.edu.cn
† dds@ustc.edu.cn
‡ drshi@ustc.edu.cn

The term "polariton" comes from the fact that Eq. 3(a) possesses bosonic commutation relations under plane-wave decomposition when the mixing angle $\theta$ satisfies $\tan\theta = g\sqrt{N}/\Omega$. By plugging Eq. S2b into Eq. S1a and substituting $\{\hat{a}_f, \hat{\sigma}_{gs}\}$ with $\{\hat{\Psi}, \hat{\Phi}\}$ one has:

$$\left(\frac{\partial}{\partial t} + c\cos^2\theta\frac{\partial}{\partial z} - \frac{ic}{2k_s}\cos^2\theta\frac{\partial^2}{\partial \rho^2}\right)\hat{\Psi}\left(\vec{\rho}, z, t\right) = -\dot{\theta}\hat{\Phi} - \sin\theta\cos\theta c\frac{\partial}{\partial z}\hat{\Phi} + \frac{ic}{2k_s}\sin\theta\cos\theta\frac{\partial^2}{\partial \rho^2}\Phi. \tag{S4}$$

Under the adiabatic limit, i.e. a sufficiently slow varying of signal and control fields, one finds $\hat{\Phi} \approx 0$ in the lowest order. Finally, by performing the following transform:

$$\tilde{\mathbf{\Psi}}\left(z, t; \vec{q}\right) = \exp\left(-i\frac{q^2 z}{2k_s}\right)\frac{1}{2\pi}\iint \hat{\Psi}\left(\vec{\rho}, z, t\right)e^{-i\vec{q}\cdot\vec{\rho}}\mathrm{d}^2\vec{\rho} \tag{S5}$$

We can eliminate the last term in the LHS of Eq. S4 and obtain a simple form of the motion equation for $\tilde{\mathbf{\Psi}}$ [2]:

$$\left(\frac{\partial}{\partial t} + v_g\frac{\partial}{\partial z}\right)\tilde{\mathbf{\Psi}}\left(z, t; \vec{q}\right) = 0. \tag{S6}$$

The above equation depicts DSPs propagating with an $\Omega$-controlled instantaneous group velocity $v_g = c\cos^2\theta = c/(1 + g^2N/\Omega^2)$. During the write-in stage, $v_g$ gradually decreases to zero as control I light adiabatically switched off while DSPs change from photon-like to spin-wave-like ($\theta \to \pi/2$) with its transverse mode preserved:

$$\tilde{a}_f\left(z = 0, t'; \vec{q}\right) \Rightarrow \sqrt{N}\tilde{\sigma}_{gs}\left(z', t; \vec{q}\right), \quad t' \in \left[0, T_s\right]. \tag{S7}$$

Eq. S7 is under the assumption of initial condition $\tilde{\sigma}_{gs}(z, 0; \vec{q}) = 0$ and $z' = \int_{t'}^{t} v_g\left(\tau\right)\mathrm{d}\tau$, here $T_s$ is signal pulse duration. We then perform the inverse transform of Eq. S5 as $\tilde{\sigma}_{gs}(\vec{\rho}, z, t) = \exp(iq^2 z/2k_s)\mathcal{F}^{-1}[\tilde{\sigma}_{gs}(z', t; \vec{q})]$ to obtain the collective atomic excitation in the laboratory coordinate, here $\mathcal{F}^{-1}$ stands for inverse Fourier transform. Since our setup satisfies $q^2 z'/2k_s \leq q^2 L/k_s \ll 1$, we can approximate the exponential term to be one. Note that $\hat{a}_f\left(0, \vec{\rho}, t\right) \propto \tilde{\mathcal{E}}\left(0, \vec{\rho}, t\right)$ and $\hat{\sigma}_{gs} = \tilde{\sigma}_{gs}U_{-l}$, therefore the mapping between signal electric field ($\mathcal{E}_s$) and atomic coherence in the write-in stage satisfies:

$$\sqrt{N}\hat{\sigma}_{gs}\left(z', \vec{\rho}, t\right) \Leftrightarrow \mathcal{E}_s\left(0, \vec{\rho}, t'\right)U_{-l}. \tag{S8}$$

After a controllable delay $t_s$, we adiabatically turn on the control II light and reach the condition $\Omega \gg g\sqrt{N}$ ($\theta \to 0$). In this read-out process, DSPs changes back to photon-like and propagate at a speed approaching $c$ till it escape from the medium as pure photons. The read-out process has the initial conditions: $\hat{a}_f^R|_{t=0} = 0$ and $\tilde{\sigma}_{gs}^R|_{t=0} = \hat{\sigma}_{gs}^W(z, \vec{\rho}, t \to \infty) \propto \mathcal{E}_{in,\perp}^W\left(\vec{\rho}\right)U_{-l}^W f\left(z\right)$, here the superscript R(W) denotes read-out(write-in). The explicit form of $f\left(z\right)$ is determined by the temporal profile of $\mathcal{E}_s$ and $\Omega$. When the control II light also carries another spiral phase $U_{l'}^W$, by rotating from $\tilde{\sigma}_{gs}^R$ back to $\hat{\sigma}_{gs}^R$ one has

$$\mathcal{E}_{out,\perp}^R \propto \mathcal{E}_{in,\perp}^W\left(\vec{\rho}\right)U_{-l}^W U_{l'}^R = \mathcal{E}_{in,\perp}^W\left(\vec{\rho}\right)U_{l'-l}. \tag{S9}$$

To this end, one anticipate from Eq. S9 that the spiral phases carried by control lights are converted to the collective atomic excitation during the write-in stage and then to retrieved signal field during the read-out stage of a memory based on EIT protocol.

## II. METHOD OF THEORETICAL SIMULATION

The $\mathrm{TEM}_{00}$ mode light fields are collimated (Thorlabs F220FC-780) before entering the experimental setup, allowing us to approximate their wavefronts as planar (the expected Rayleigh length $\approx 4.4 \times 10^3$ m significantly exceeds the beam waist). We then apply a spiral phase $\exp(il\phi)$ to the control field's wavefront through via the SLM (see FIG. 1 (b) in the main text). Consequently, the modulated light field belongs to a subfamily of well-studied hyper-Geometric Gaussian (HyGG) modes [3]. This light field can generally be expanded in terms of Laguerre-Gaussian modes characterized by the same azimuthal index $l$ and varying radial indices $p$ (denoted as $\mathrm{LG}_p^l$):

$$U_{\mathrm{HyGG}}^l = g\left(\vec{\boldsymbol{r}}\right)\exp\left(il\phi\right) = \sum_p c_p \mathrm{LG}_p^l\left(\vec{\boldsymbol{r}}\right). \tag{S10}$$

Therefore, HyGG modes are not free-space eigen modes and thus do not exhibit propagation invariance. For example, FIG. S1(a) illustrates the theoretical beam profiles of different topological charges $l$ during diffraction from the SLM to the center of the MOT, guided by a $4f$ imaging system. It is evident that there is a hole around the phase singularity that increases with the

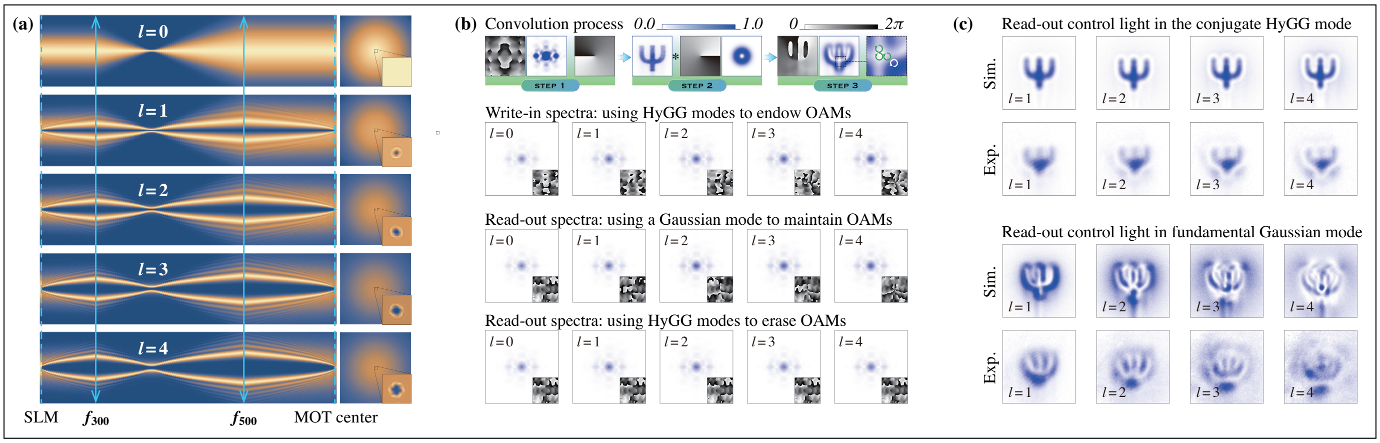


FIG. S1. Simulation using HyGG modes. (a) Diffraction of control light fields on their way to the MOT cell, where size of the 4f lens group is set as 25 mm. (b) Theoretical signal pattern, Fourier spectrum, and corresponding spectra with different HyGG modes in write-in and read-out stages. (c) Comparison of theoretical simulation and experimental results of secondary convolution during the read-out stage, where the second and the fourth row show images retrieved from memory using identical HyGG and Gaussian control light, respectively.

topological charge due to high-frequency leakage. These holes contribute to a highlighted outline around the retrieved patterns in FIG. 3(a) and result in a drop in quantum efficiency during all-optical convolutions, as demonstrated in FIG. 3(c) of the main text. We utilize the above profiles of the control field in the MOT center as the point spread function and perform convolution calculations. FIG. S1 (b) presents the schematic of simulation (the first row), write-in spectra of the signal image using HyGG mode control light with different $l$ (the second row), the readout spectra using a Gaussian mode to keep the spiral phase (the third row) or HyGG modes to wipe out the spiral phase (the fourth row) carried by spectra. These simulated results in the Fourier plane clearly demonstrate the maintenance or erasure of spiral phases, as expected from Equation S9. Additionally, FIG. S1(c) shows the retrieved images from memory, using control lights in various HyGG modes or fundamental Gaussian modes. By spatially integrating these patterns, we obtain the simulated retrieval efficiencies, which are presented in FIG. 3(c) of the main text and align with the experimental results. To clarify the simulation process without losing generality, we provide a specific example where $l = 1$, as depicted in the first row of FIG. S1(b). We simplify the form of the modulated control light field imaged into the MOT center as follows: $U_c(r,\phi) \propto \exp(il\phi)\exp[-r^2/w_0^2]$, where $w_0$ is the waist of the control field. Ignoring the finite aperture of the lenses, the diffracted field on the back focal plane (which coincides with the ICCD) can be expressed as:

$$U_c(\rho,\theta) \propto (-i)^{l+1}\exp(il\theta)\sqrt{\pi}\frac{w_0}{\rho_0}\frac{\rho}{\rho_0}\exp\left(-\frac{\rho^2}{\rho_0^2}\right)\times\left[I_{\frac{l-1}{2}}\left(\frac{\rho^2}{\rho_0^2}\right)-I_{\frac{l+1}{2}}\left(\frac{\rho^2}{\rho_0^2}\right)\right]. \tag{S11}$$

Here $\rho_0^2 = 2\lambda^2 f_2^2/(\pi^2 w_0^2)$ is the square of effective radius that increases with $f_2$ and decreases with $w_0$, $\lambda$ is the wavelength of the control light and $I_\alpha(x)$ stands for the $\alpha$th-order modified Bessel function of the first kind. This doughnut-shaped field (see FIG. S1(b), step 2) resembles the Laguerre-Gaussian mode with azimuthal index $l$ and radial index 0. Even though the dependence of storage-retrieval efficiency on the intensity of coupling lights is quite complicated, we still use Eq. S11 in the following simulation for a qualitative understanding. As indicated by Eq. S9, when using a control light with $U_l^W = \exp(i\phi)$ in the write-in stage and a plane wave control light ($U_{l'}^R = 1$) in the read-out stage, the retrieved signal field on ICCD approximates to the convolution of mask pattern with the optical vortex $U_c$, and thus we come to a simulation result shown in the step 3 of FIG. S1 (b). The phenomenon of edge enhancement arises from the destructive interference between two adjacent points in the uniform area of the retrieved signal field, the conditions for which are not satisfied in the presence of intensity or phase jumps.

## III. EXPERIMENTAL DETAILS

*Preparation of magnetically insensitive states.* — At the beginning of each experimental cycle, we ensure that the majority of atoms occupy state $|5S_{1/2}, F = 2, m_F = 0\rangle$ (denoted as $|g\rangle$) by simultaneously illuminating the ensemble with $\pi$-polarized light that is tuned to resonate with the $|g\rangle \leftrightarrow |5P_{1/2}, F' = 2\rangle$ transition and two beams of state preparation (SP) light target the $|5S_{1/2}, F = 3\rangle\,(|s\rangle) \leftrightarrow |5P_{1/2}, F' = 2\rangle$ transition [4]. A strong guiding magnetic field, aligned with the quantization axis, lifts the degeneracy of the Zeeman sub-levels. The accumulation of atoms in the desired state is due to the fact that the $\pi$-transition from $|g\rangle$ to $|5P_{1/2}, F' = 2, m_{F'} = 0\rangle$ has a corresponding Clebsch-Gordan coefficient of zero, making it dipole-forbidden [5]. We optimize the efficiency of state preparation by finely adjusting the detuning of SP lights to match the strength of the applied magnetic field (see the supplemental material of [6]). During the write-in stage, when the signal light and the control light are

orthogonally linearly polarized, the photonic information is mapped as Zeeman coherence between $|g\rangle$ and $|s, m_{F'} = 0\rangle$. This coherence is resilient to decoherence caused by ambient magnetic fields. Thus, it is called a magnetically-insensitive state [7].

*Frequency filtering and data acquisition systems.* — A filter composed of a Glan-Taylor polarizer and a rubidium absorption cell is positioned in front of the ICCD to eliminate the control light while maintaining the transverse mode of the readout signal light. Alternatively, the absorption cell and ICCD can be replaced with a set of Fabry–Pérot etalons and a photomultiplier tube to capture the temporal profile of the signal light collected through a multimode fiber (as shown in FIG. 1 (c) of the main text, for example). It is crucial to ensure the collinearity of the signal and control fields; any misalignment will introduce a spatially dependent phase term to the collective excitation. We collimate the signal and control beams using a single-mode fiber before inserting lens $f_3$, and then we adjust the position of $f_3$ based on the retrieved pattern to meet the necessary requirements.

*Time sequence.* — The experiment is conducted at a repetition rate of 40 Hz. At the start of each experimental cycle, a repumping light, resonant with the transition $\left|5S_{1/2}, F = 2\right\rangle \leftrightarrow \left|5P_{3/2}, F' = 3\right\rangle$, is activated for $19.5\,ms$. A red-detuned cooling light ($-20$MHz), targeting the transition $\left|5S_{1/2}, F = 3\right\rangle \leftrightarrow \left|5P_{3/2}, F' = 4\right\rangle$, is turned off $500\,\mu s$ after the repumping light is switched off. As a result, most atoms in the ensemble end up in the $\left|5S_{1/2}, F = 2\right\rangle$state by the end of the cooling process. The magnetic field for trapping atoms remains on until the cooling light is turned off, and the magnetic field for guiding is switched on $200\,\mu s$before the trapping field begins to deactivate, and this guiding field stays on for the entire duration of the experimental window. This timing sequence allows for a sufficiently long build-up time of the guiding field prior to the start of the experimental window while not significantly impacting the cooling process of the magneto-optical trap, provided that the repetition frequency of the experiments is maintained. The trapping and guiding magnetic fields are manipulated by absorbing circuits consisting of high-speed MOSFETs. The trapping and guiding magnetic fields are controlled by absorbing circuits that utilize high-speed MOSFETs. The experimental window opens $300\,\mu s$ after the trapping field starts to switch off, during which all three beams of state preparation lights are turned on for 30 $\mu s$ at the beginning of each window. The signal pulse to be stored lasts for $800\,ns$ and is emitted into the ensemble within the experimental window. Control pulses in the write-in stage and read-out stage, both lasting $3\,\mu s$, are used in the experiment. The storage time $\tau_s$ is defined as the interval between the falling edge of the write-in control pulse and the rising edge of the read-out control pulse. We optimize storage efficiency by carefully adjusting the moment when the control light is diabatically switched off. In the read-out stage, the counter-propagating pumping light in the heated absorption cell is turned off to minimize unwanted scattering noise, as illustrated in FIG. 1(b) of the main text.


[1] M. Fleischhauer and M. D. Lukin, Quantum memory for photons: Dark-state polaritons, Phys. Rev. A **65**, 022314 (2002).

[2] T. Golubeva, Y. Golubev, O. Mishina, A. Bramati, J. Laurat, and E. Giacobino, High-speed spatially multimode atomic memory, Phys. Rev. A **83**, 053810 (2011).

[3] E. Karimi, G. Zito, B. Piccirillo, L. Marrucci, and E. Santamato, Hypergeometric-gaussian modes, Opt. Lett. **32**, 3053 (2007).

[4] B. Wang, Y. Han, J. Xiao, X. Yang, C. Zhang, H. Wang, M. Xiao, and K. Peng, Preparation and determination of spin-polarized states in multi-zeeman-sublevel atoms, Phys. Rev. A **75**, 051801 (2007).

[5] J. J. Sakurai and J. Napolitano, *Modern quantum mechanics* (Cambridge University Press, 2020).

[6] Y.-H. Ye, L. Zeng, M.-X. Dong, W.-H. Zhang, E.-Z. Li, D.-C. Li, G.-C. Guo, D.-S. Ding, and B.-S. Shi, Long-lived memory for orbital angular momentum quantum states, Phys. Rev. Lett. **129**, 193601 (2022).

[7] B. Zhao, Y.-A. Chen, X.-H. Bao, T. Strassel, C.-S. Chuu, X.-M. Jin, J. Schmiedmayer, Z.-S. Yuan, S. Chen, and J.-W. Pan, A millisecond quantum memory for scalable quantum networks, Nature Phys. **5**, 95 (2009).
